# Supplementary material for: Ordering-Based Causal Structure Learning in the Presence of Latent Variables
Source: arXiv:1910.09014 source file (2020-03-24)
Supplement: Supplementary file 1 [file appendix.tex]

\documentclass[twoside]{article}

\usepackage[accepted]{aistats2020}
\usepackage{xcolor}
\usepackage{algorithm}
\usepackage{algpseudocode}
\usepackage{subcaption}
\usepackage{graphicx}
\usepackage[titletoc, title]{appendix}

% If your paper is accepted, change the options for the package
% aistats2020 as follows:
%
% \usepackage[accepted]{aistats2020}

% If you use natbib package, activate the following three lines:
\usepackage[round]{natbib}
\bibliographystyle{plainnat}

% If you use BibTeX in apalike style, activate the following line:

\usepackage{tikz,calc}

\input{cbs_defs}

%\externaldocument{template}
% In your preamble
 
\usepackage{xr}

\makeatletter
\newcommand*{\addFileDependency}[1]{% argument=file name and extension
  \typeout{(#1)}
  \@addtofilelist{#1}
  \IfFileExists{#1}{}{\typeout{No file #1.}}
}
\makeatother
 
\newcommand*{\myexternaldocument}[1]{%
    \externaldocument{#1}%
    \addFileDependency{#1.tex}%
    \addFileDependency{#1.aux}%
}

\myexternaldocument{main}
% just to see what's happening

\begin{document}

\twocolumn[
\aistatstitle{
Supplementary Material: Ordering-Based Causal Structure Learning \\in the Presence of Latent Variables
}
\aistatsauthor{ Daniel Irving Bernstein$^*$ \And Basil Saeed$^*$ \And Chandler Squires$^*$ \And Caroline Uhler}
\aistatsaddress{ MIT \And MIT \And MIT \And MIT} ]
\appendix

\input{appendix_text.tex}

\bibliographystyle{plainnat}  
\bibliography{references}  %%% Remove comment to use the external .bib file (using bibtex).

\end{document}
